# Supplementary material for: AlphaRouter: Quantum Circuit Routing with Reinforcement Learning and Tree Search
Source: arXiv:2410.05115 source file (2024-10-07)
Supplement: Supplementary file 1 [file appendix.tex]

\section{Supplementary Materials}\label{sec:appendix}

\subsection{Quantum Computer Topology}
\begin{figure}[t]
% \vskip 0.2in
\begin{center}
\centerline{\includegraphics[width=.35\columnwidth]{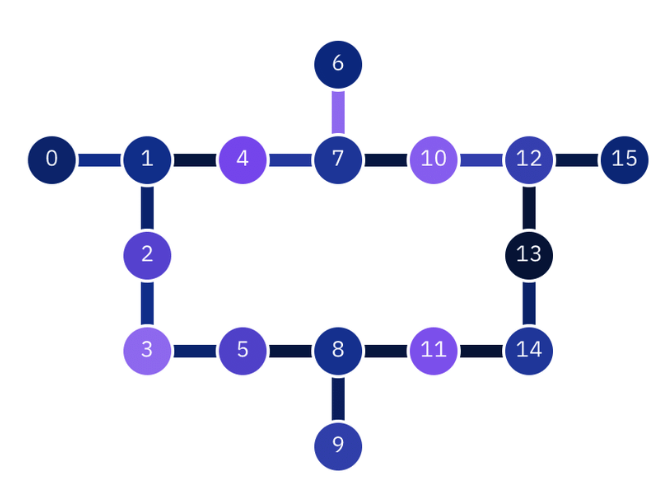}}
\caption{The IBM Guadalupe quantum computer.}
\label{fig:guadalupe}
\end{center}
\vskip -0.2in
\end{figure}

Quantum computer topology, particularly in the realm of superconducting quantum computers~\cite{barends2014superconducting}, is a critical aspect that significantly influences their operational capabilities and design. Superconducting quantum computers, which are among the leading technologies in quantum computing, are characterized by their unique physical architecture where qubits are arranged in a specific pattern or layout. A defining feature of these systems is that they primarily allow for interactions between nearest neighbor qubits. This means that a quantum gate operation can be directly performed only between adjacent qubits in the physical layout. This nearest neighbor interaction constraint is a key consideration in quantum circuit design and compilation, as it necessitates additional steps, like the insertion of SWAP gates, to facilitate interactions between non-adjacent qubits. Optimizing quantum circuit operations within the bounds of this topological structure is crucial for the effective implementation and scaling of superconducting quantum computers.

Figure~\ref{fig:guadalupe} displays the topology of the IBM Guadalupe quantum computer, where the physical qubits are numbered from $0$ to $15$. This topology is structured in a heavy hexagon configuration, which is conducive to the application of efficient quantum error correction codes, enhancing the system's overall fault tolerance and computational reliability.

Besides superconducting qubits, several other leading technologies are at the forefront of quantum computing, each with its unique topological challenges. For instance, trapped ion quantum computers~\cite{ospelkaus2011microwave,kielpinski2002architecture} use ions trapped in electromagnetic fields as qubits. While they typically support interactions between distant qubits, they face challenges in scaling and maintaining accuracy as the number of qubits increases. Photonic quantum computers~\cite{loss1998quantum}, which utilize photons for computation, excel in stability and scalability but grapple with challenges in ensuring reliable interactions between photons and in error correction. Each of these technologies must contend with specific topological limitations and operational challenges, influencing their development pathways and potential applications in the quantum computing landscape.

\subsection{Quantum Computing Compilation}
Quantum computing compilation involves several key components that translate high-level quantum algorithms into executable instructions on Quantum Processing Units (QPUs). Initially, the process starts with \textbf{Algorithm Representation}~\cite{nielsen2001quantum}, where quantum algorithms are expressed as logical quantum circuits using quantum gates and qubits. Next, in the \textbf{Circuit Optimization}~\cite{gokhale2020optimized} phase, these circuits are simplified and optimized for performance, often through gate fusion, cancellation, or other techniques to reduce complexity. The \textbf{Qubit Mapping or Routing}~\cite{shafaei2014qubit} stage then deals with aligning the logical qubits from the circuit with the physical qubits on the QPU, a step made challenging by limited qubit connectivity in most quantum hardware. This often requires the insertion of SWAP gates to rearrange qubits into configurations permissible by the hardware topology. \textbf{Decomposition}~\cite{shende2005synthesis} follows, where complex multi-qubit gates are broken down into simpler, hardware-supported gates. Finally, the \textbf{Scheduling and Control} phase involves determining the precise timing and sequence of gate operations, considering the constraints and latencies of the quantum hardware. Throughout these stages, error mitigation and correction strategies may also be integrated to enhance the reliability of quantum computations. This entire compilation process is crucial in bridging the gap between theoretical quantum algorithms and practical execution on quantum hardware.
